# Supplementary material for: Federated Learning with Nesterov Accelerated Gradient
Source: arXiv:2009.08716 source file (2022-10-26)
Supplement: Supplementary file 1 [file appendixG.tex]

\section{Proof of \texorpdfstring{$\cos{\theta}\geq0$}{cos(theta)>=0} when \texorpdfstring{$\eta\to0^+$}{eta to 0+} (Observation \texorpdfstring{\textcircled{1}}{1} in Theorem 4)}
\label{appendixG}
\begin{proof}
When $\eta\to0^+$, recalling the definition of $p$, %$p \triangleq \max _{k\in [1,K], t \in[k]} \frac{\left\|\gamma\mathbf{v}_{[k]}(t)\right\|}{\left\|\eta\nabla F\left(\mathbf{w}_{[k]}(t)\right)\right\|}$, 
we can get $\|\gamma \mathbf{v}_{[k]}(t)\| \leq p \|\eta \nabla F(\mathbf{w}_{[k]}(t))\|\simeq0$. Then, We have $\Vert\mathbf{v}_{[k]}(t)\Vert\simeq0,\mathbf{v}_{[k]}(t)\simeq\mathbf{0}$. Thus, we have
\begin{flalign*}
&-2\nabla F(\mathbf{w}_{[k]}(t))^{\mathrm{T}} \mathbf{v}_{[k]}(t)=\Vert\nabla F(\mathbf{w}_{[k]}(t))\Vert^2+\Vert\mathbf{v}_{[k]}(t)\Vert^2\\
&\quad-\Vert\mathbf{v}_{[k]}(t)+\nabla F(\mathbf{w}_{[k]}(t))\Vert^2\simeq0.
\end{flalign*}
Therefore, $\cos \theta_{[k]}(t)\simeq0$ for any $k\in[1, K]$ and $t\in[k]$, which proves $\cos{\theta}\geq0$.
\end{proof}
