# Supplementary material for: Federated Learning with Nesterov Accelerated Gradient
Source: arXiv:2009.08716 source file (2022-10-26)
Supplement: Supplementary file 3 [file appendix_notation.tex]

\section{Notation Summary}
\label{appendix:notation}
\begin{table}[hbt!]
\centering
\caption{Notation summary}
\label{tab:notation}
\begin{tabular}{lp{0.8\columnwidth}}
\hline
$i$ & index of worker \\
$t$ & index of update iteration \\
$k$ & index of interval \\
$N$ & number of workers\\
$T$ & number of total local iterations\\
$K$ & number of global aggregations\\
$D_i$ & number of samples for local dataset $i$\\
$D$ & total number of samples\\
$\eta$ & learning step size hyper parameter \\
$\gamma$ & momentum hyper parameter \\
$\tau$ & number of local update steps between two global aggregations \\
%$\delta_i$ & upper bound between $\nabla F_i(\mathbf{w})$ and $\nabla F(\mathbf{w})$ \\ 
%$[k]$ & interval $[(k-1)\tau, k\tau]$ \\
$F(\mathbf{w})$ & global loss function\\
$F_i(\mathbf{w})$ & local loss function for worker $i$\\
$\mathbf{w}^{\mathrm{f}}$        & practical model parameter that the learning process can obtain \\
$\mathbf{w}^*$         & theoretical model parameter that minimizes $F(\mathbf{w})$ \\
$\mathbf{w}(t)$         & global model parameter at iteration $t$ \\
$\mathbf{w}_i(t)$ & local model parameter at iteration $t$ for worker $i$ \\
%$\Tilde{\mathbf{w}}_i(t)$ & local model parameter at iteration $t$ for worker $i$ after possible global aggregation \\
$\mathbf{v}(t)$ &  global momentum parameter at iteration $t$\\
$\mathbf{v}_i(t)$ & local momentum parameter at iteration $t$ for worker $i$\\
%$\Tilde{\mathbf{v}}_i(t)$ & local momentum parameter at iteration $t$ for worker $i$ after possible global aggregation\\
$\mathbf{w}_{[k]}(t)$ & model parameter for centralized NAG at iteration $t$ in interval $[k]$ \\
$\mathbf{v}_{[k]}(t)$ & momentum parameter for centralized NAG at iteration $t$ in interval $[k]$ \\
%$\theta_{[k]}(t)$ & angle between vector negative gradient $-\nabla F(\mathbf{w}_{[k]}(t))$ and $\mathbf{v}_{[k]}(t)$ \\
%$\theta$ & the maximum value of $\theta_{[k]}(t)$ for $1\leq k\leq K$ with $t \in [k]$\\
\hline
\end{tabular}
\end{table}
